# Supplementary material for: Understanding the Robustness of Randomized Feature Defense Against Query-Based Adversarial Attacks
Source: arXiv:2310.00567 source file (2023-10-01)
Supplement: Supplementary file 1 [file supp.tex]

This Appendix provides additional details, analysis, and experimental results to support the main paper. We begin by discussing the limitations in Section~\ref{sec:limitations} and societal impacts in Section~\ref{sec:impacts}. Then, we provide the proof for Theorem 1 in the main paper in Section~\ref{sec:proofs}. Next, the detailed experimental setup is provided in Section~\ref{sec:setup}, which is followed by additional robustness experiments to demonstrate the effectiveness of the proposed defense. Finally, we provide additional visualization of the robust behavior of the models with randomized features in Section~\ref{sec:visualization}.

\section{Limitations} \label{sec:limitations}
% As discussed, we focus on studying the effectiveness of the feature-space randomized defense on ViT under score-based attacks. Our analysis does not apply to decision-based attacks, which find adversarial samples from just hard labels given by the model.
% \hl{anything about decision-based attacks?}. 
As discussed, we focus on studying the effectiveness of the randomized feature defense for DNNs against black-box attacks, including score-based and decision-based attacks. We do not include black-box attacks that utilize the transferability from surrogate to target models since our threat model does not make any assumptions about the network architecture and the training dataset. 

Our proposed defense adds another layer of protection to DNNs against adversarial attacks, and it would be interesting to study the adversarial robustness of the combination of our randomized feature defense and existing defense strategies, including those that have been developed for transfer-based attacks~\cite{pang2019improving,tramer2017ensemble,yang2020dverge}.  We leave these to future works.

\section{Societal Impacts} \label{sec:impacts}

Deep neural networks (DNN) rapidly transform our daily lives in various domains and applications. Unfortunately, most well-trained DNNs are vulnerable to adversarial attacks, which decreases confidence in their deployment. Among the existing adversarial attacks, query-based attacks pose a severe threat to users since these attacks are effective and only require access to the model's feedback; the attackers do not know the trained parameters or model architectures. 

Our work tackles this defense challenge against query-based attacks by proposing a lightweight adversarial defense for existing DNNs. We conduct a detailed theoretical analysis of our defense and show its superior performance compared to other randomized defenses in extensive empirical experiments across a wide range of DNN architectures, query-based attacks, and benchmark datasets. Most importantly, our method can be directly integrated into any existing off-the-shelf DNN. In summary, the proposed randomized feature defense can boost the adversarial robustness of existing DNNs against most query-based attacks, further improving the users's confidence when using them in practice. 

\section{Proof of Section~3.2} \label{sec:proofs}
% \begin{theorem}\label{thm:robustness}
\robustness*
    % Assuming the proposed random vector $u$ is sampled from a Gaussian $\Ncal(0, \mu I)$, the model is decomposed into $f=g\circ h$, and the defense adds a random noise $\delta\sim\Ncal(0, \nu I)$ to the output of $h$. At input $x$, the probability that the attacker chooses an opposite action positively correlates with \[\arctan\left(-\left(\frac{2\nu}{\mu}\frac{\|\nabla_{h(x)} (\mathcal{L}\circ g)\|^2_2}{\|\nabla_x (\mathcal{L}\circ f)\|^2_2}\right)^{-0.5}\right).\]

% \end{theorem}
\begin{proof}
    For score-based attacks, the attacker finds the direction by computing $\Lcal(f(x + u)) -\Lcal(f(x))$. When applying randomized defense, the direction instead relies on $\Lcal(\randf(x+u)) - \Lcal(\randf(x))$. As discussed in Section~3, the probability that the attacker chooses an opposite action is 
    \begin{equation}
        \mathbb{P}\left[\frac{\Lcal(\randf(x+u)) - \Lcal(\randf(x))}{\Lcal(f(x + u)) -\Lcal(f(x))}<0\right].
    \end{equation}
    If the defense adds a random noise $\delta\sim\Ncal(0, \nu I)$ to the output of layer $h$ of the model $f=g\circ h$, we have $\Lcal(\randf(x)) = \Lcal(g(h(x)+\delta)$. Since $\delta$ and $u$ are small, we can linearly approximate the objection function
    \begin{align}
        \Lcal(f(x+u))&\approx \Lcal(f(x)) + \nabla_x(\Lcal\circ f)^{\intercal}u ,\\
        \Lcal(g(h(x)+\delta)&\approx\Lcal(f(x)) + \nabla_{h(x)}(\Lcal\circ g)^{\intercal}\delta,\\
        \Lcal(g(h(x+u)+\delta)&\approx\Lcal(g(h(x)+J_h(x)u + \delta)\\
        &\approx\Lcal(f(x))+ \nabla_{h(x)}(\Lcal\circ g)^{\intercal}J_h(x)u + \nabla_{h(x)}(\Lcal\circ g)^{\intercal}\delta\\
        &= \Lcal(f(x)) + \nabla_x(\Lcal\circ f)^{\intercal}u +\nabla_{h(x)}(\Lcal\circ g)^{\intercal}\delta,
        \end{align}
    where $\nabla_{h(x)}(\Lcal\circ g)$ is the gradient of $\Lcal\circ g$ evaluated at $h(x)$, $\nabla_x(\Lcal\circ f)$ is the gradient of $\Lcal\circ f$ at $x$, $J_h(x)$ is the Jacobian matrix of $h$ at $x$.

    At a different application of $\randf$, the randomized model samples a new noise vector. Let $\delta_1, \delta_2$ be the sampled noises when querying $\Lcal(\randf(x+u))$ and $\Lcal(\randf(x))$, the ratio can be approximated by 
    \begin{align}
        \frac{\Lcal(\randf(x+u)) - \Lcal(\randf(x))}{\Lcal(f(x + u)) -\Lcal(f(x))}&\approx \frac{\nabla_x(\Lcal\circ f)^{\intercal}u +\nabla_{h(x)}(\Lcal\circ g)^{\intercal}\delta_1 - \nabla_{h(x)}(\Lcal\circ g)^{\intercal}\delta_2}{\nabla_x(\Lcal\circ f)^{\intercal}u}\\
        &= 1 + \frac{\nabla_{h(x)}(\Lcal\circ g)^{\intercal}(\delta_1 - \delta_2)}{\nabla_x(\Lcal\circ f)^{\intercal}u}.
    \end{align}
    Since $\delta_1$ and $\delta_2$ are independent, we have $\delta_1 - \delta_2 \sim\Ncal(0, 2\nu I)$, thus
    \begin{align}
        \nabla_{h(x)}(\Lcal\circ g)^{\intercal}(\delta_1 - \delta_2)&\sim\Ncal(0, 2\nu\|\nabla_{h(x)}(\Lcal\circ g)\|_2^2),\\
        \nabla_x(\Lcal\circ f)^{\intercal}u&\sim\Ncal(0, \mu \|\nabla_x(\Lcal\circ f)\|_2^2).
    \end{align}

    The noises $\delta_1, \delta_2$ added by the defense and the noise $u$ added by the attacker are independent, therefore the ratio of two independent normal variable $\frac{\nabla_{h(x)}(\Lcal\circ g)^{\intercal}(\delta_1 - \delta_2)}{\nabla_x(\Lcal\circ f)^{\intercal}u}$ follows Cauchy distribution with location $0$ and scale $\sqrt{\frac{2\nu}{\mu}}\frac{\|\nabla_{h(x)} (\mathcal{L}\circ g)\|_2}{\|\nabla_x (\mathcal{L}\circ f)\|_2}$. In this case, the probability that the attacker is fooled can be approximated by
    \begin{align}
        \mathbb{P}\left[\frac{\Lcal(\randf(x+u)) - \Lcal(\randf(x))}{\Lcal(f(x + u)) -\Lcal(f(x))}<0\right]&\approx \mathbb{P}\left[\frac{\nabla_{h(x)}(\Lcal\circ g)^{\intercal}(\delta_1 - \delta_2)}{\nabla_x(\Lcal\circ f)^{\intercal}u}<-1\right]\\
        &= \frac{1}{\pi}\arctan\left(-\left(\frac{2\nu}{\mu}\frac{\|\nabla_{h(x)} (\mathcal{L}\circ g)\|^2_2}{\|\nabla_x (\mathcal{L}\circ f)\|^2_2}\right)^{-0.5}\right) + \frac{1}{2}.
    \end{align}
\end{proof}

\section{Experimental Setup} \label{sec:setup}
\subsection{Dataset}
In this work, we conduct experiments on two widely used datasets in adversarial attacks, CIFAR10 and ImageNet. We randomly selected $1000$ images per dataset such that the test sets cover all classes, each of which has equal size.
\begin{itemize}
    \item \textbf{CIFAR10}\footnote{\url{https://www.cs.toronto.edu/~kriz/cifar.html}} consists of $60,000$ images from 10 different classes where the training set has $50,000$ images and the test set has $10,000$ images.  
    \item \textbf{ImageNet (ILSVRC) 2012}\footnote{\url{https://www.image-net.org/download.php}} is a large-scale dataset that consists of $1000$ classes. The training set includes $1,281,167$ images, the validation set includes $50,000$ images, and the test set has $100,000$ images. 
\end{itemize}

For all experiments, we resize the images to $224\times 224$ resolution. 
\subsection{Models}
As discussed in the main text, we consider $4$ models that have various architectures, including ResNet50~\cite{He2016resnet}, VGG19~\cite{Simonyan2015vgg}, ViT base~\cite{dosovitskiy2020image}, DeiT base~\cite{touvron21a2021deit}. We use the pretrained weights from \verb|timm| package\footnote{\url{https://github.com/huggingface/pytorch-image-models}} for ImageNet, and finetune ResNet50, VGG19, ViT base, DeiT base for CIFAR10.
\subsection{Implementation of the Black-box Attacks}
We perform experiments on $3$ score-based black box attacks (Square attack~\cite{andriushchenko2020square}, NES~\cite{ilyas2018black}, and Signhunter~\cite{al2020sign}) and $2$ decision-based attacks (RayS~\cite{chen2020rays} and SignFlip~\cite{Chen2020boosting}). For $\ell^{\infty}$ attacks, we find adversarial samples within the $\ell^{\infty}$ ball of radius $0.05$, for $\ell^2$ attacks we set the radius to $5$. The detailed hyperparameters of each attack are as follows:
\begin{itemize}
    \item \textbf{Square attack}: The initial probability of pixel change is $0.05$ for $\ell^{\infty}$ attack and $0.1$ for $\ell^2$ attack.\\
    \item \textbf{NES}: We estimate the gradient by finite difference with $60$ samples for $\ell^{\infty}$ attack and $30$ for $\ell^2$ attack. The step size of finite difference is $0.01$ and $0.005$, and the learning rate is set to $0.005$ and $1$ for $\ell^{\infty}$ and $\ell^2$ attack, respectively.
\end{itemize}
\subsection{Evaluation}
According to Section~3, a sample is considered as adversarial if it can fool the model in the majority of its application. Since the randomized model has stochasticity, for any datapoint there is a chance that the prediction is flipped at some application. Therefore, an attacker can stop the attack before finding the true adversarial sample. To alleviate this issue, when deciding whether to stop the attack, the query is repeated multiple times, and the attack is considered to be successful if the prediction is consistently flipped in most of the runs. The experiment applies $9$ query runs for verification, and these extra runs are not included in the total number of queries. 

\section{Additional experiments} \label{sec:additional_experiments} 
\subsection{Performance against $\ell^2$ Attacks}
We provide the results of randomized feature defense against $\ell^2$ attacks on CIFAR10 in Table~\ref{tab:l2_cifar10}. As we can observe, $\ell^2$ attacks are quite successful in fooling the model; however, randomized feature defense improves the robustness of the models to these attacks.
\begin{table}[h!]
    \caption{The robustness against $\ell^2$ attacks on CIFAR10.}
    \label{tab:l2_cifar10}
    \centering
    \begin{tabular}{lllcccccc}
        \toprule
         \multirow{2}{*}{Model} & \multirow{2}{*}{Method}  & \multirow{2}{*}{Acc} & 
         \multicolumn{2}{c}{Square} &
        \multicolumn{2}{c}{NES} &
        \multicolumn{2}{c}{SignHunter} \\
        % \cline{4-9} 
        \cmidrule(l){4-5}\cmidrule(l){6-7} \cmidrule(l){8-9}
        &&& 1000 & 10000 &1000 & 10000 & 1000 & 10000\\
        \midrule
         \multirow{2}{*}{VGG19} & Base &96.28 & 13.5 & 3.0 & 72.9 & 50.7 & 44.2 & 11.2\\
         & Feature & 93.58& 85.3 & 82.8 & 91.4 & 87.9 & 87.1 & 85.7 \\
         \midrule
         \multirow{2}{*}{ViT} & Base & 97.86& 48.5 & 28.6 & 87.8 & 73.5 & 60.7 & 30.3 \\
         & Feature & 93.38 & 88.2 & 88.1 & 92.7 & 90.1& 86.4 & 85.7\\
         \bottomrule
    \end{tabular}
    
\end{table}
% \subsection{Adversarial training}
\subsection{Performance against Decision-based Attacks}
Table~\ref{tab:dec_imagenet} shows the performance of the model on ImageNet under decision-based attacks. Similar to CIFAR10, randomized feature defense is effective against decision-based attacks while AAA~\cite{chen2022aaa} defense is not helpful in this case, since decision-based attacks only rely on the label that the model returns and AAA defense keeps the output label be the same.
\begin{table}[h!]
    \centering
    \caption{The robustness against decision-based attacks on ImageNet.}
     \begin{tabular}{lll|cc}
        \toprule
         Model & Method & Acc & RayS & SignFlip \\
         \midrule 
        \multirow{4}{*}{VGG19} & Base & 74.21 & 0.1 & 1.0  \\
        & AAA & 74.24 & 0.4 & 0.8  \\
        & Input & 71.43 & 6.6 & 53.3   \\
        & Feature & 71.21 & 10.0 & 46.9 \\
        \midrule
        \multirow{4}{*}{ViT} & Base & 79.15 & 1.7 & 9.7  \\
        & AAA &  79.14 & 2.2 & 9.7  \\
        & Input & 77.09 & 41.3 &  70.3 \\
        & Feature & 77.18 &  41.0 & 70.1  \\
        
        \bottomrule
         
    \end{tabular}
    
    \label{tab:dec_imagenet}
\end{table}

\noindent \textbf{AAA's Performance against score-based attacks.} We also provide the evaluation of AAA under score-based attacks in Table~\ref{tab:aaa}. Since AAA is optimized for score-based attacks directly, it is successful in fooling the attack.  However, under a general setting where the defender does not know the type of attack is currently performed (a more realistic scenario), AAA failed miserably as shown above, while our defense performs well regardless of the attack.
\begin{table}[h]
    % \scriptsize
    % \setlength{\tabcolsep}{1pt}
    \centering
    \caption{Robustness against score-based attacks of AAA (CIFAR10).}
    \begin{tabular}{@{}l|ccc|ccc@{}}
    \toprule
    \multirow{2}{*}{Attack} & \multicolumn{3}{c|}{VGG19} & \multicolumn{3}{c}{ViT} \\
                            & Input   & AAA   & Feature  & Input  & AAA  & Feature \\ \midrule
    Square                  & 18.7    & 27.1  & 23.3     & 61.3   & 66.6 & 63.7    \\
    NES                     & 47.4    & 58.6  & 55.1     & 70.6   & 73.7 & 72.2    \\ \bottomrule
    \end{tabular}
    \label{tab:aaa}
\end{table}

\subsection{Performance against White-box Attacks}
As mentioned in the main paper, similar to previous works~\cite{byun2022effectiveness, qin2021random, chen2022aaa}, our threat model focuses on defending against black-box, query-based attacks, as it is a more realistic scenario in practice. Nevertheless, in this section, we provide an additional study about the performance of our defense against white-box attacks, those that require access to the model's architecture and its parameters. We evaluate the performance of our method against C\&W~\cite{carlini2017towards} and PGD~\cite{madry2017towards} with $\ell_{\infty}$ constraint $\epsilon=0.03$. As observed in Table~\ref{tab:whitebox}, the proposed defense can boost the robustness against these white-box attacks while having a negligible degradation in clean accuracy. We conjecture that adding stochasticity to the model can transform it into a smoothed classifier and therefore reduce the adversarial effect. 

% our analysis in Section~\ref{main_part} is not applicable to white-box attacks, previous works~\cite{liu2018towards, he2019parametric, cohen2019certified} show that adding stochasticity to the model can transform it into a smoothed classifier and therefore reduce adversarial effect. 

% We evaluate the performance of our method under white-box attacks, which are C\&W~\cite{carlini2017towards} and PGD~\cite{madry2017towards} with $\ell_{\infty}$ constraint $\epsilon=0.03$; and report the accuracy under attack on CIFAR10 in Table~\ref{tab:whitebox}, which implies that randomized feature defense can also boost the robustness to white-box attacks with negligible degradation in the clean accuracy in some circumstances.
% }
% \begin{table}[]
\begin{wraptable}{l}{0.5\textwidth}
\centering
\caption{Accuracy under white-box attacks of randomized feature defense on CIFAR10}
\begin{tabular}{@{}llccc@{}}
\toprule
Model & Method  & Acc   & C\&W    & PGD   \\ \midrule
VGG19 & Base    & 96.28 & 7.35  & 3.71  \\
      & Feature & 94.93 & 34.93 & 6.06  \\ \midrule
ViT   & Base    & 97.86 & 39.23 & 1.65  \\
      & Feature & 95.96 & 55.11 & 26.01 \\ \bottomrule
\end{tabular}
\label{tab:whitebox}
% \end{table}
\end{wraptable}
\subsection{Robustness characteristics of layers}

As discussed in Section~3.3 in the main paper, the gradient norm varies during the sequence of queries of an attack on an input. Figure~\ref{fig:vgg_ratio} suggests that, in deeper layers, the ratio of the gradient norm increases during the attack, which is related to the model’s robustness as seen in Theorem~\ref{thm:robustness}; thus the model becomes more resilient to black-box attacks. Here, we additionally provide the performance evaluation on CIFAR10 with 1000 attack queries when each layer is perturbed alone (with $\nu$ such that the clean accuracy drops within a similar threshold), as well as the mean rate of change in the gradient norm’s ratios during the sequence of queries. Table~\ref{tab:layerwise_selected_scale} implies that deeper layers induce higher change and lead to better robustness, which confirms our analysis.

\begin{table}
% \setlength{\tabcolsep}{1pt}
% \renewcommand{\arraystretch}{0.7}
% \scriptsize
\centering
\caption{Robustness (CIFAR10) at each layer with $\nu$ corresponding to $\approx 4\%$ clean accuracy drop.}
\begin{tabular}{@{}llcccc@{}}
\toprule
Model & Layer & Square & NES  & SignHunt & \begin{tabular}{@{}c@{}}
    Change of\\ Ratio
\end{tabular} \\ \midrule
VGG & 1  & 41.0   & 90.7 & 28.7 & 0.959 \\
    & 8  & 68.9 & 90.7 & 46.4 & 1.273 \\
    & 12 & 63.3 & 89.4 & 46.1 & 1.364 \\
    & 15 & 55.9 & 87.4 & 41.1 & 1.318 \\ \midrule
ViT & 1  & 67.5 & 89.7 & 17.6 & 1.089 \\
    & 4  & 69.0 & 90.2 & 24.0 & 1.692 \\
    & 8  & 69.5 & 89.8 & 37.2 & 1.751 \\
    & 11 & 78.0 & 92.7 & 43.9 & 1.728 \\ \bottomrule
\end{tabular}
\label{tab:layerwise_selected_scale}
\end{table}

\section{Behavior of Models with Randomized Features} \label{sec:visualization}
\subsection{The ratio of the norm of the gradient}
We report the ratio $\frac{2\nu}{\mu}\frac{\|\nabla_{h(x)} (\mathcal{L}\circ g)\|^2_2}{\|\nabla_x (\mathcal{L}\circ f)\|^2_2}$ before and after perturbed at hidden layers of VGG19 and ViT on ImageNet/CIFAR10 in Figure~\ref{fig:vgg_ratio} and \ref{fig:vit_ratio}. The results show that, on both datasets, when the perturbed sample moves close to adversarial samples, the probability that randomized feature defense can fool the attacker increases while the probability of randomized input defense does not change. This explains the effectiveness of randomized feature defense against score-based attacks. 
Figure~\ref{fig:vit_ratio} shows this ratio on ViT. On ImageNet, the robustness of the defense still increases during the attack; however, on CIFAR10, such behaviors between the original and perturbed samples are not significantly different.
\begin{figure}
     \centering
     \begin{subfigure}{0.5\textwidth}
         \centering
         \includegraphics[width=\textwidth]{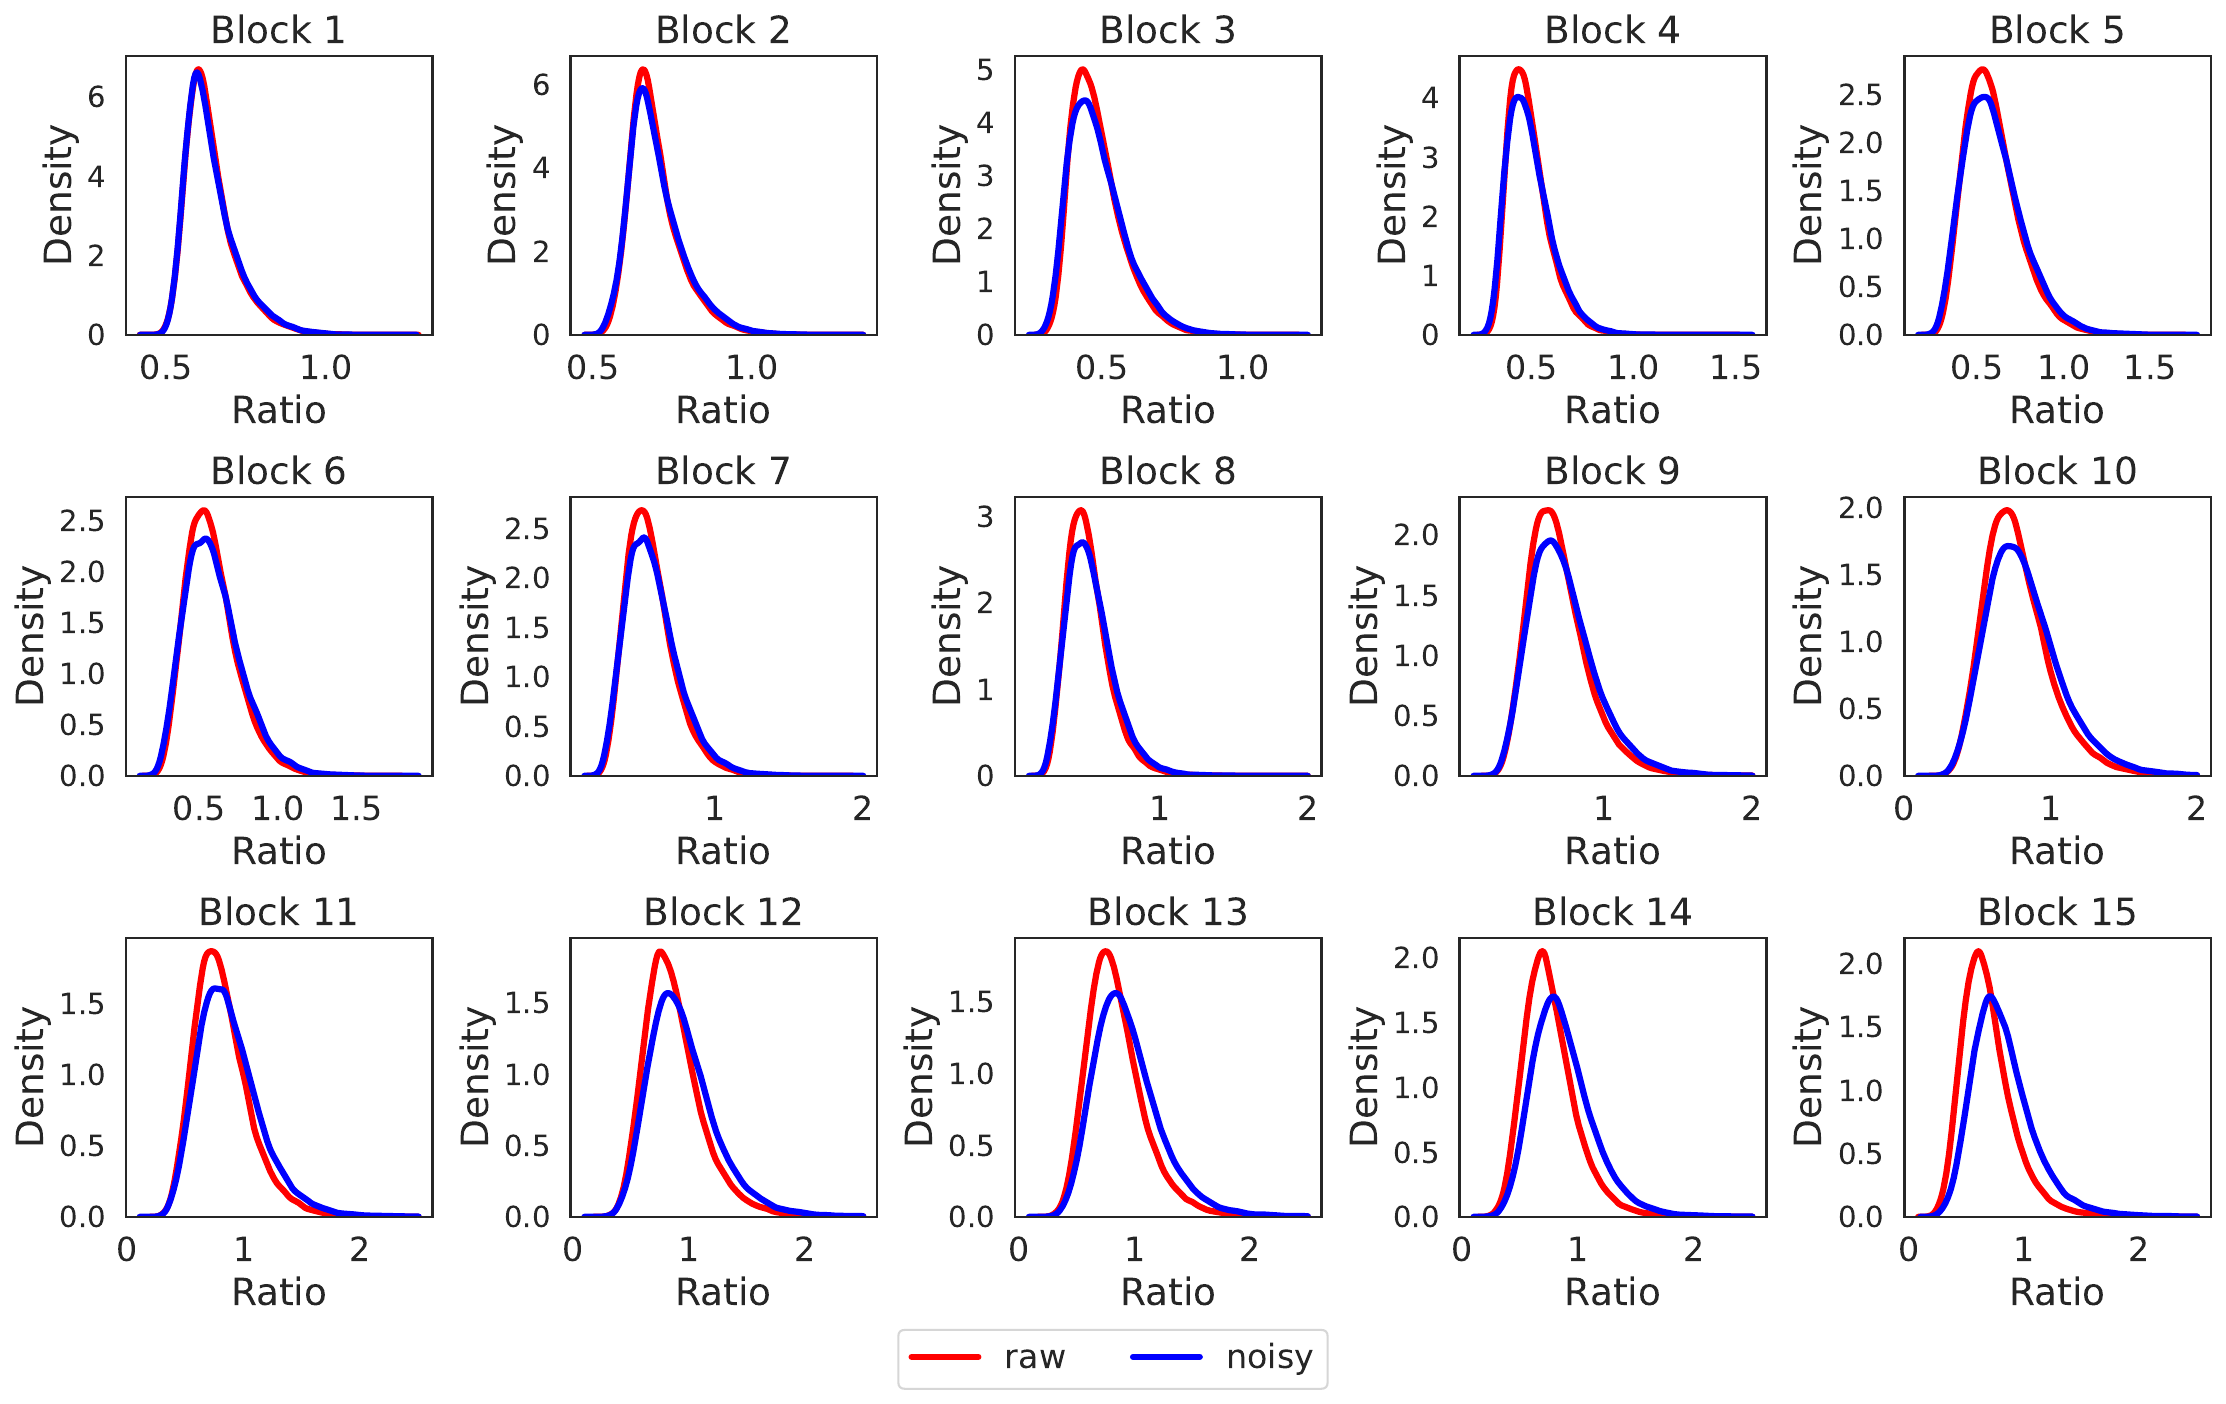}
         \caption{ImageNet}
         \label{fig:vgg_imagenet_ratio}
     \end{subfigure}%
     % \vfill
     \begin{subfigure}{0.5\textwidth}
         \centering
         \includegraphics[width=\textwidth]{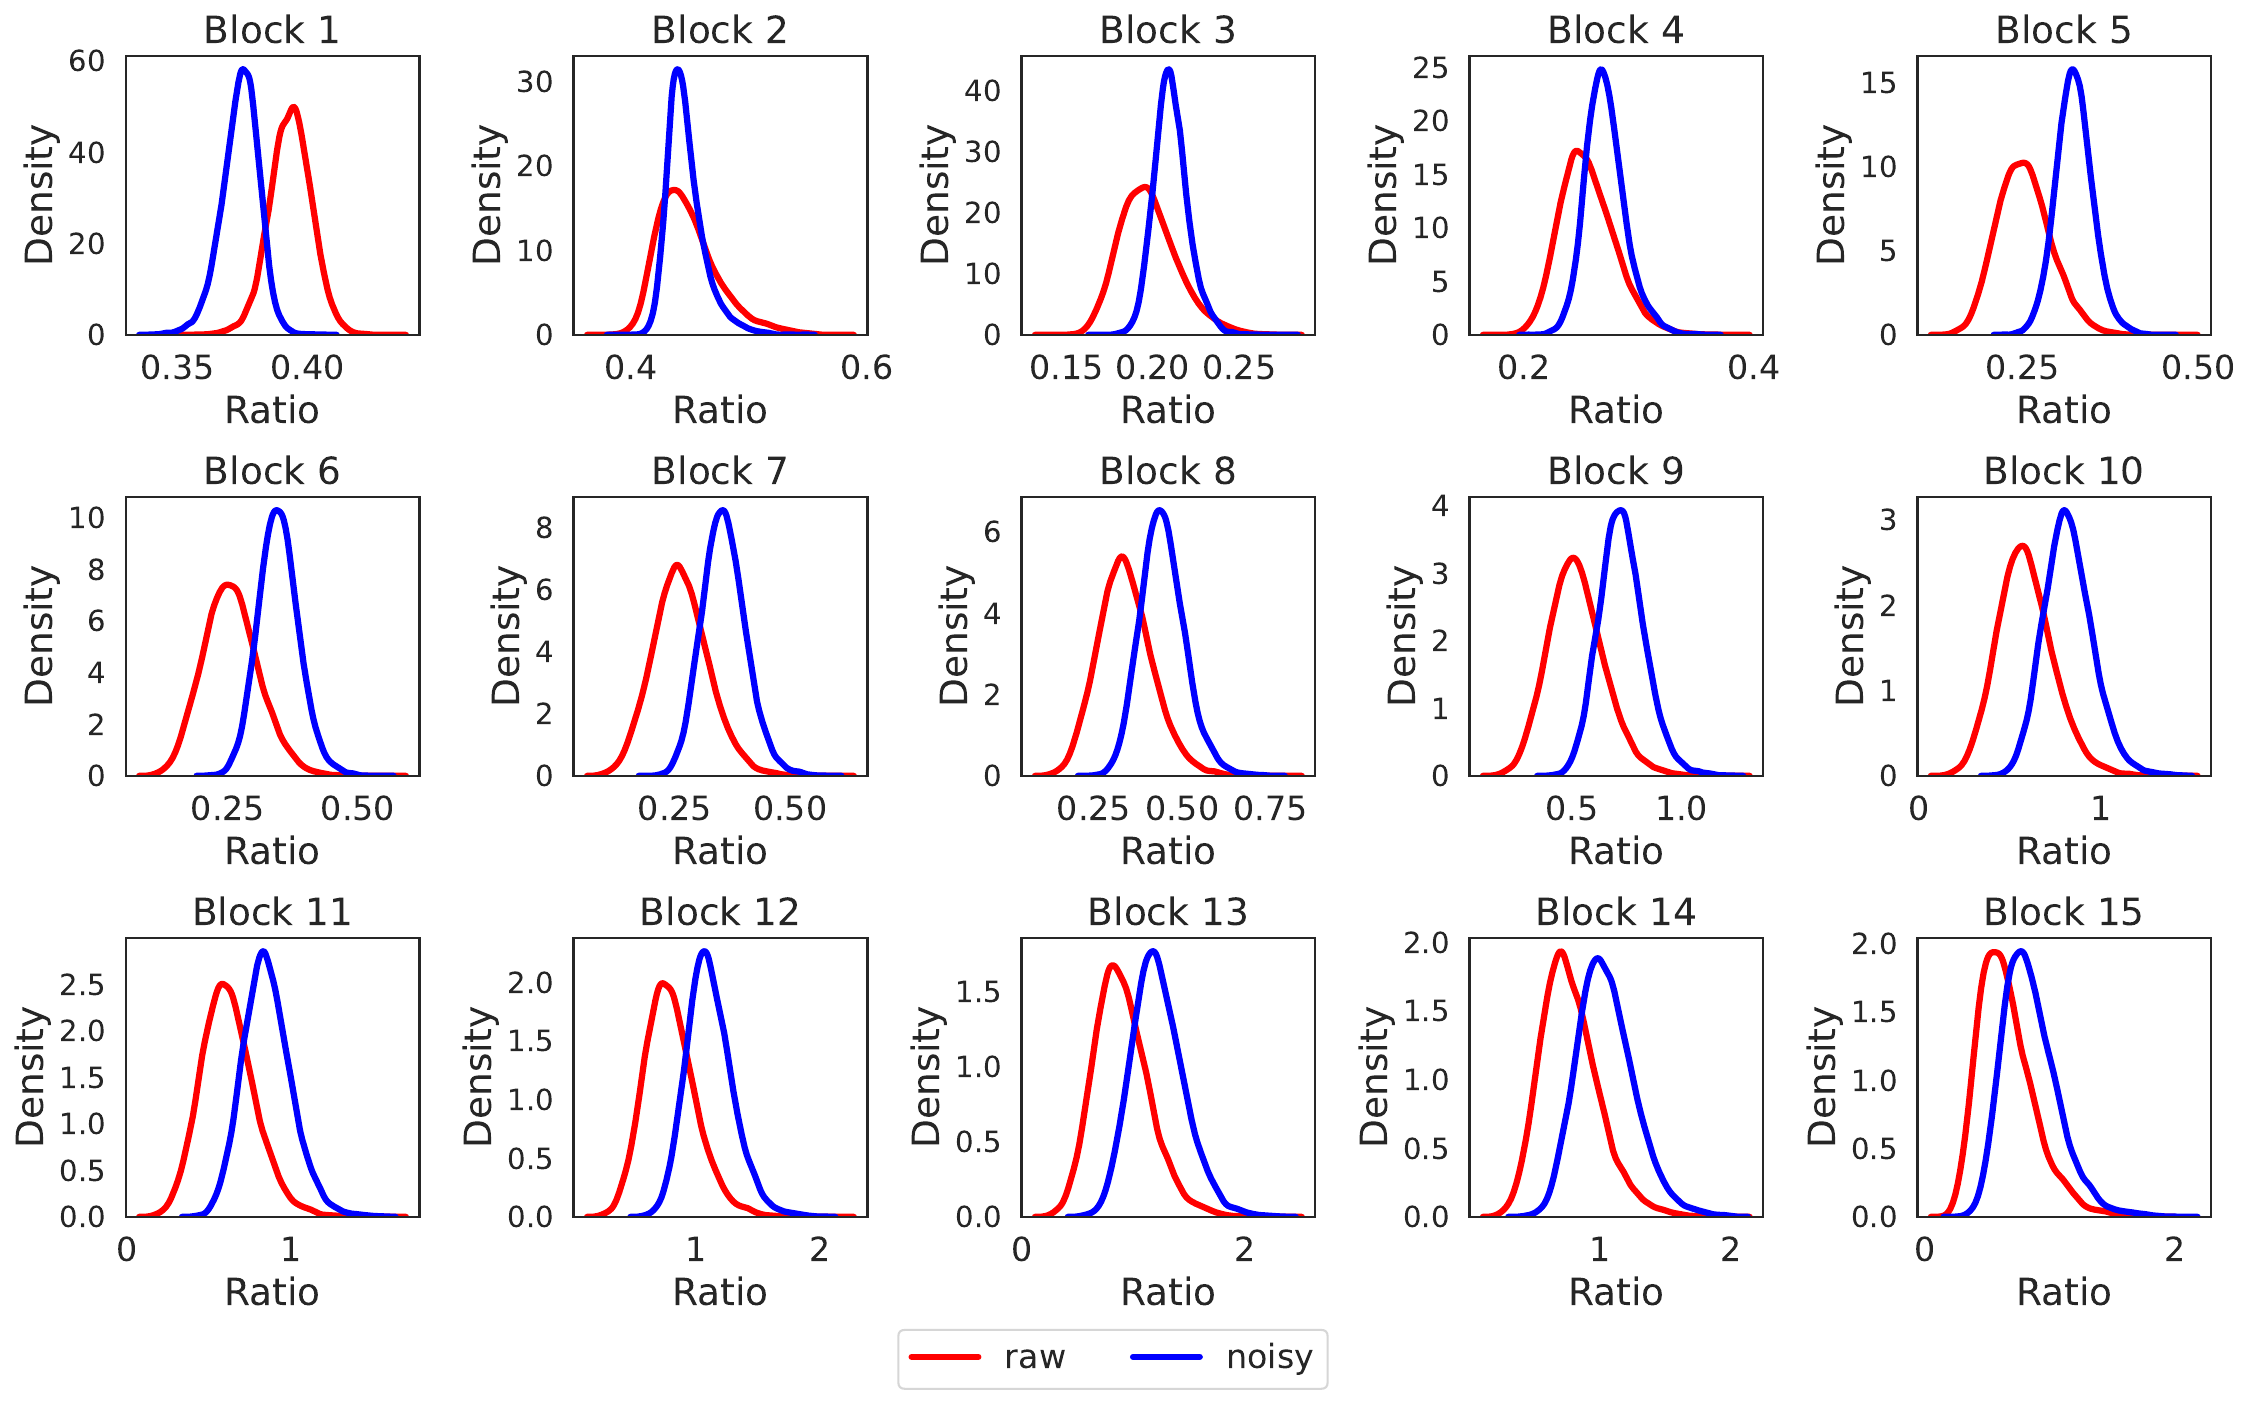}
         \caption{CIFAR10}
         \label{fig:vgg_cifar_ratio}
     \end{subfigure}
     \hfill
        \caption{The ratio of the norm of the gradient of $\Lcal$ at hidden layers and at input of VGG19 on ImageNet/CIFAR10 before and after perturbed}
        \label{fig:vgg_ratio}
\end{figure}

\begin{figure}
     \centering
     \begin{subfigure}{0.5\textwidth}
         \centering
         \includegraphics[width=\textwidth]{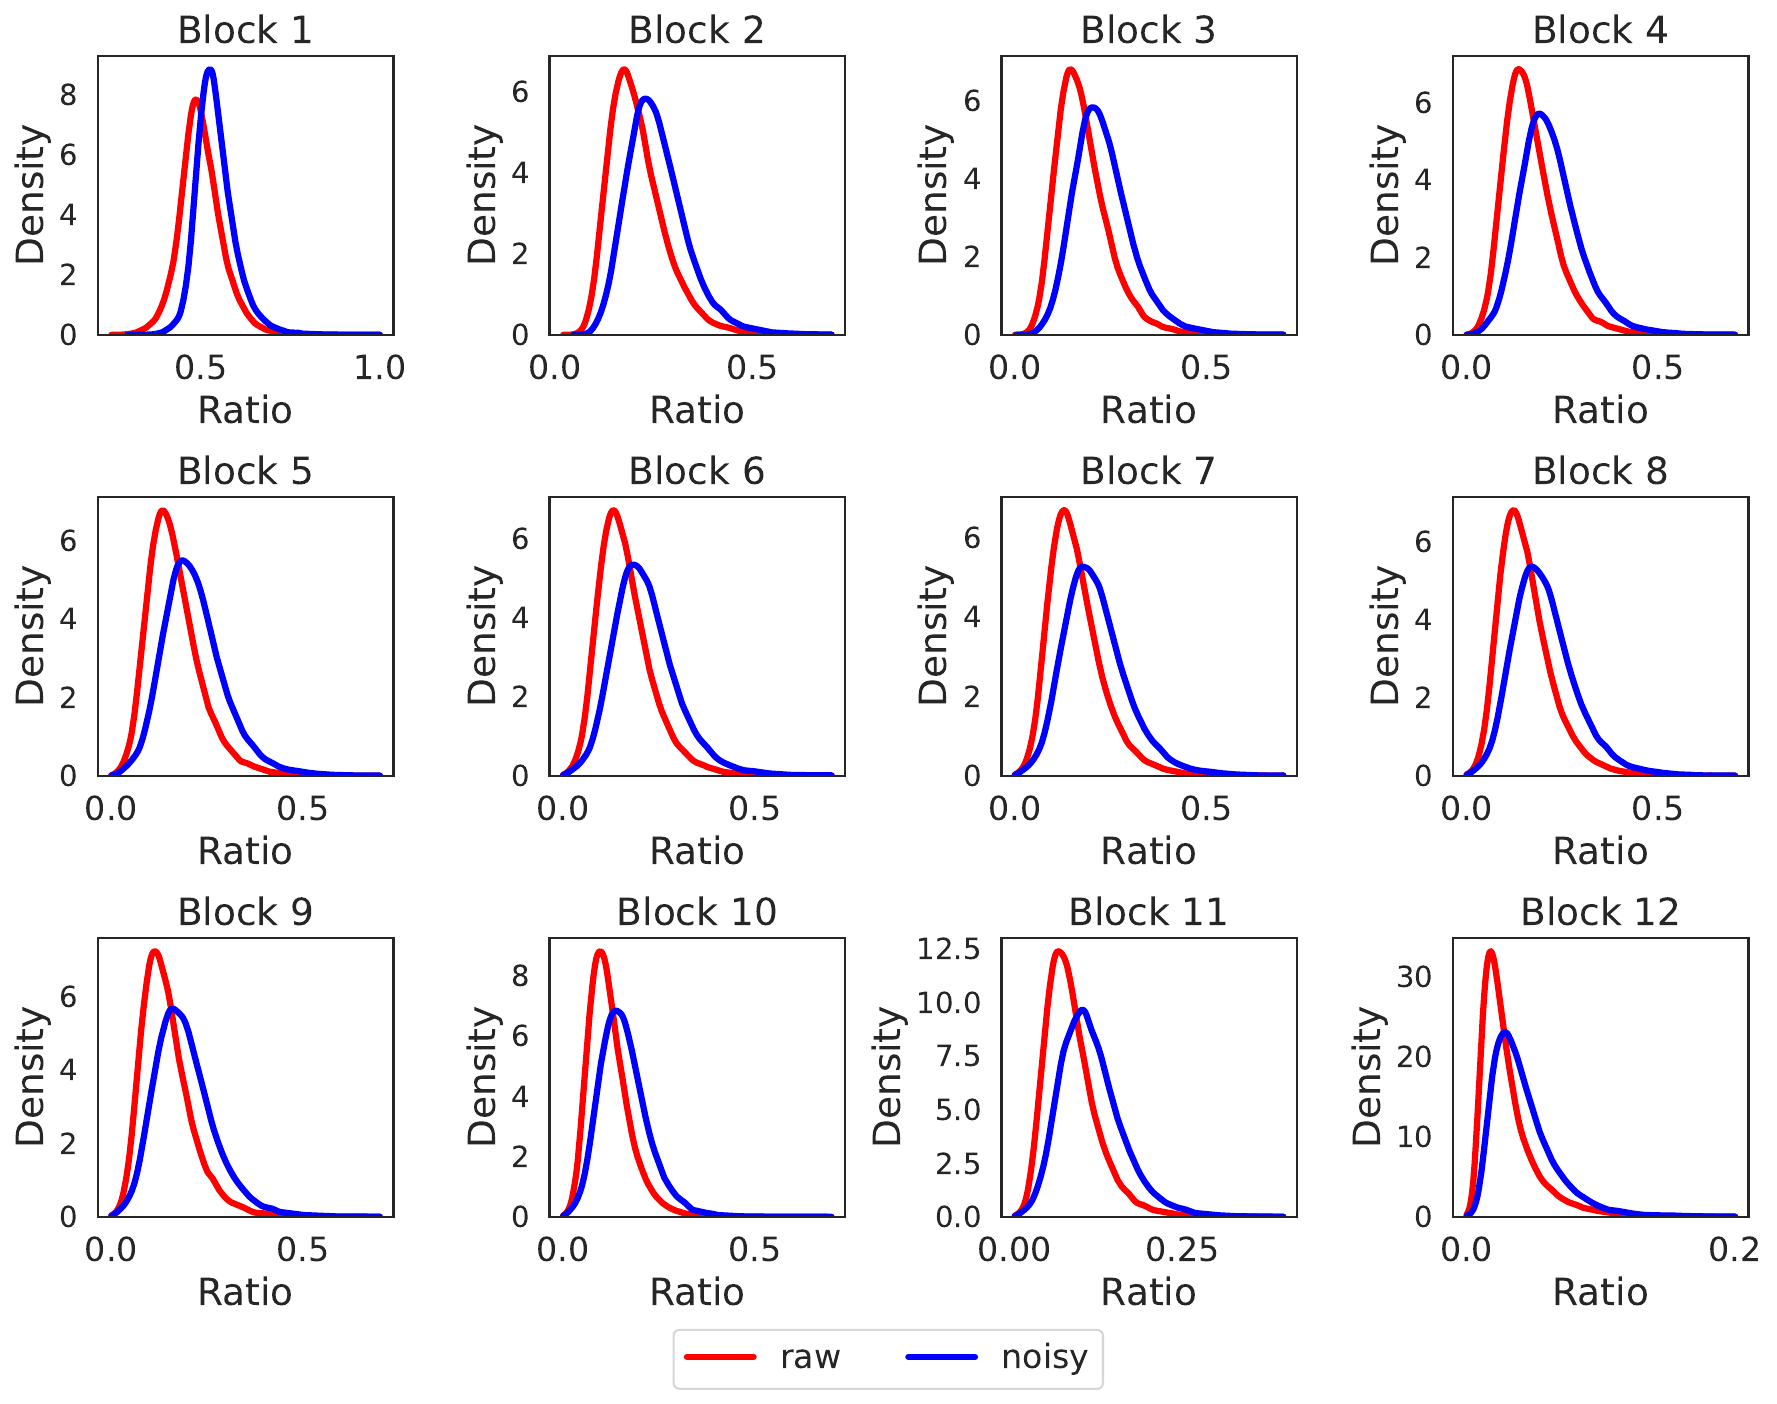}
         \caption{ImageNet}
         \label{fig:vit_imagenet_ratio}
     \end{subfigure}%
     % \vfill
     \begin{subfigure}{0.5\textwidth}
         \centering
         \includegraphics[width=\textwidth]{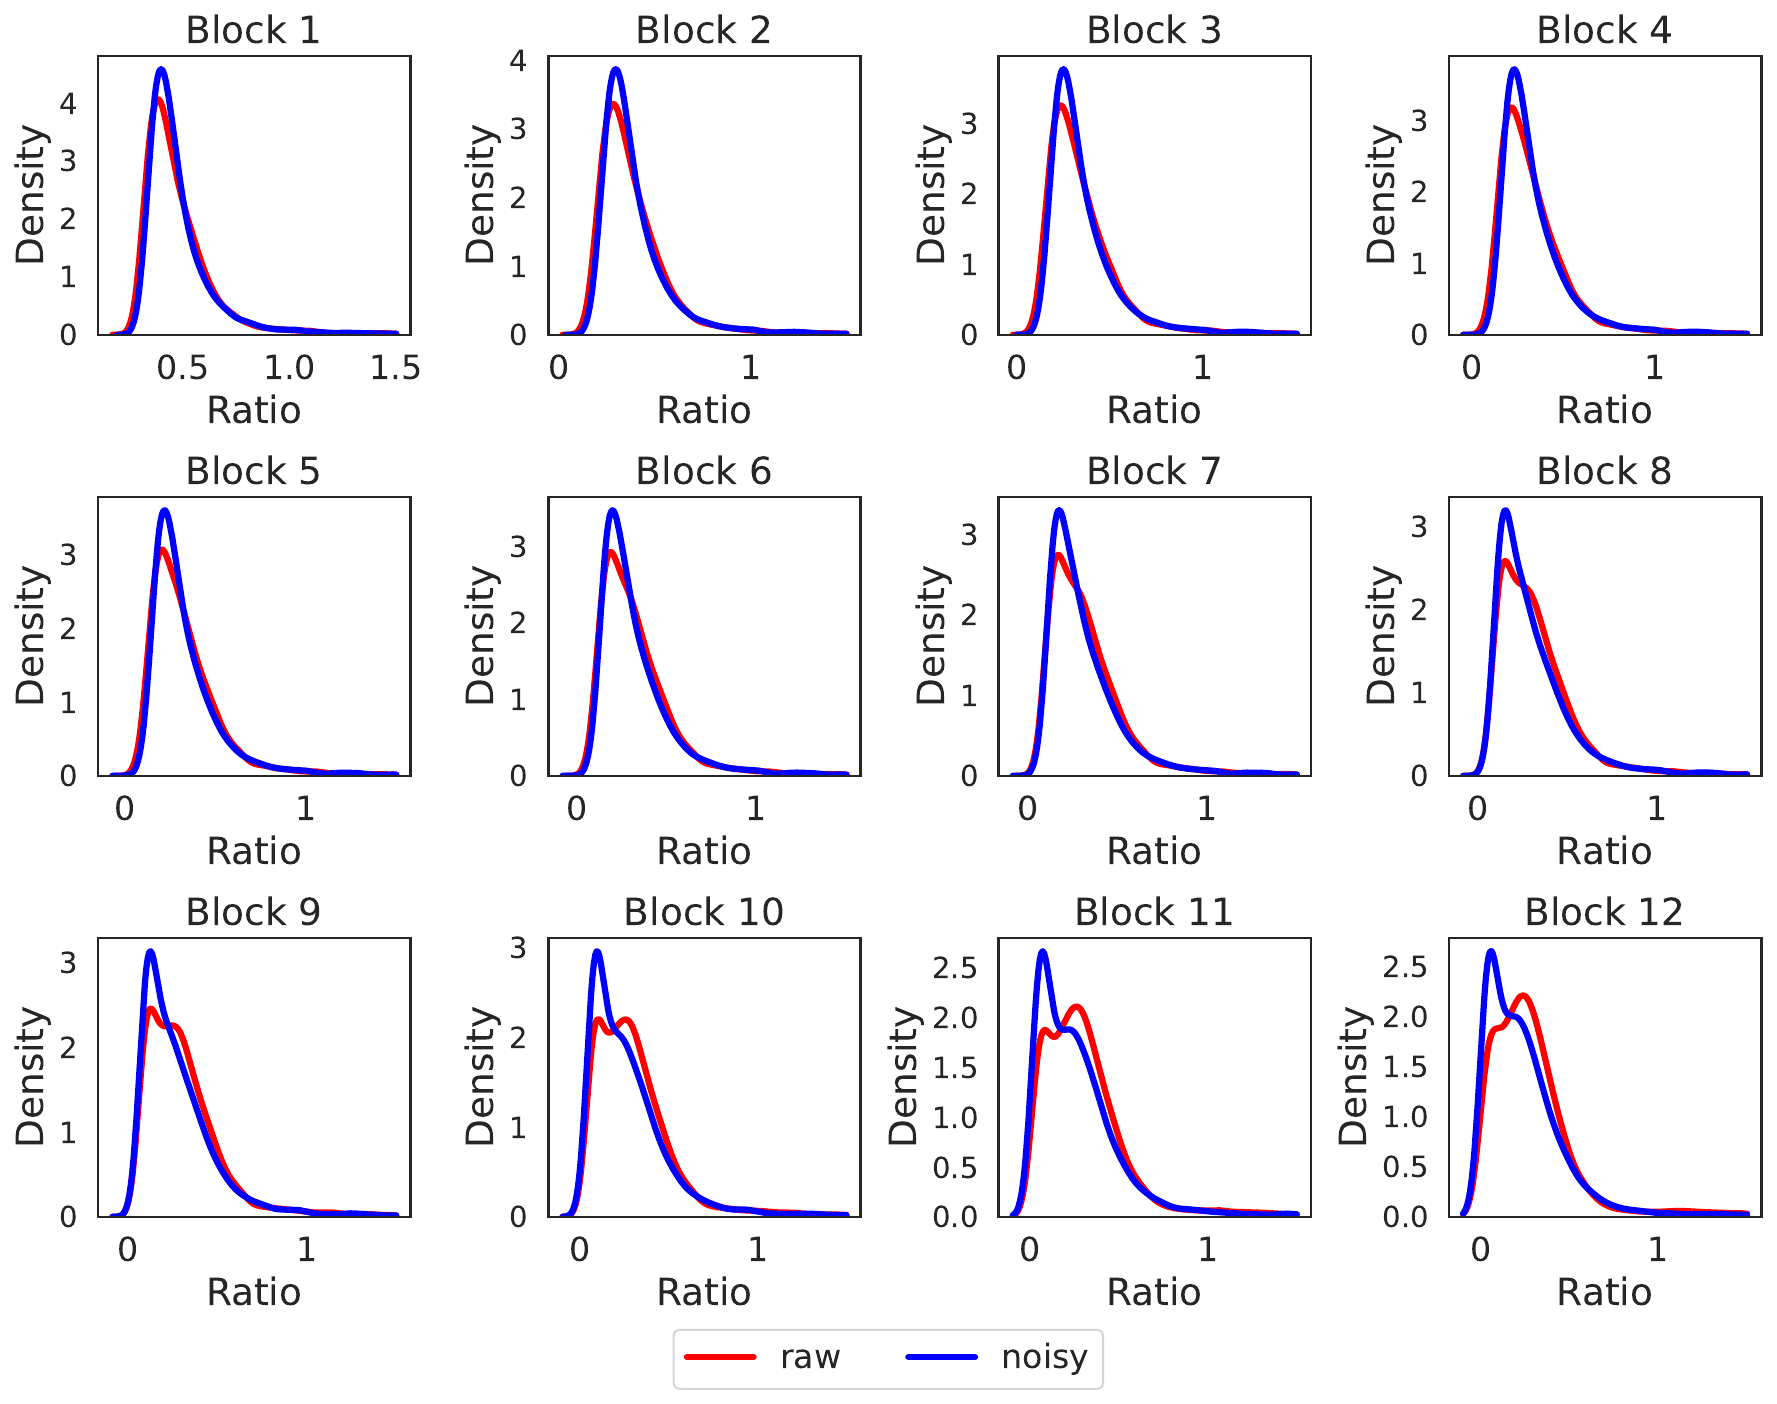}
         \caption{CIFAR10}
         \label{fig:vit_cifar_ratio}
     \end{subfigure}
     \hfill
        \caption{The ratio of the norm of the gradient of $\Lcal$ at hidden layers and at input of ViT on ImageNet/CIFAR10 before and after perturbed}
        \label{fig:vit_ratio}
\end{figure}
\subsection{The magnitude of the robustness at input and hidden layers}
Figure~\ref{fig:vgg_acc} and \ref{fig:vit_acc} show the robustness of randomized feature and randomized input defenses by multiplying the norm of the gradient with the relative magnitude of the defense noise. As we can observe, the robustness when injecting noise to the hidden layers is generally higher than when injecting noise in the input. Such robustness behaviors are more visible in the deeper layers.
\begin{figure}
     \centering
     \begin{subfigure}{0.5\textwidth}
         \centering
         \includegraphics[width=\textwidth]{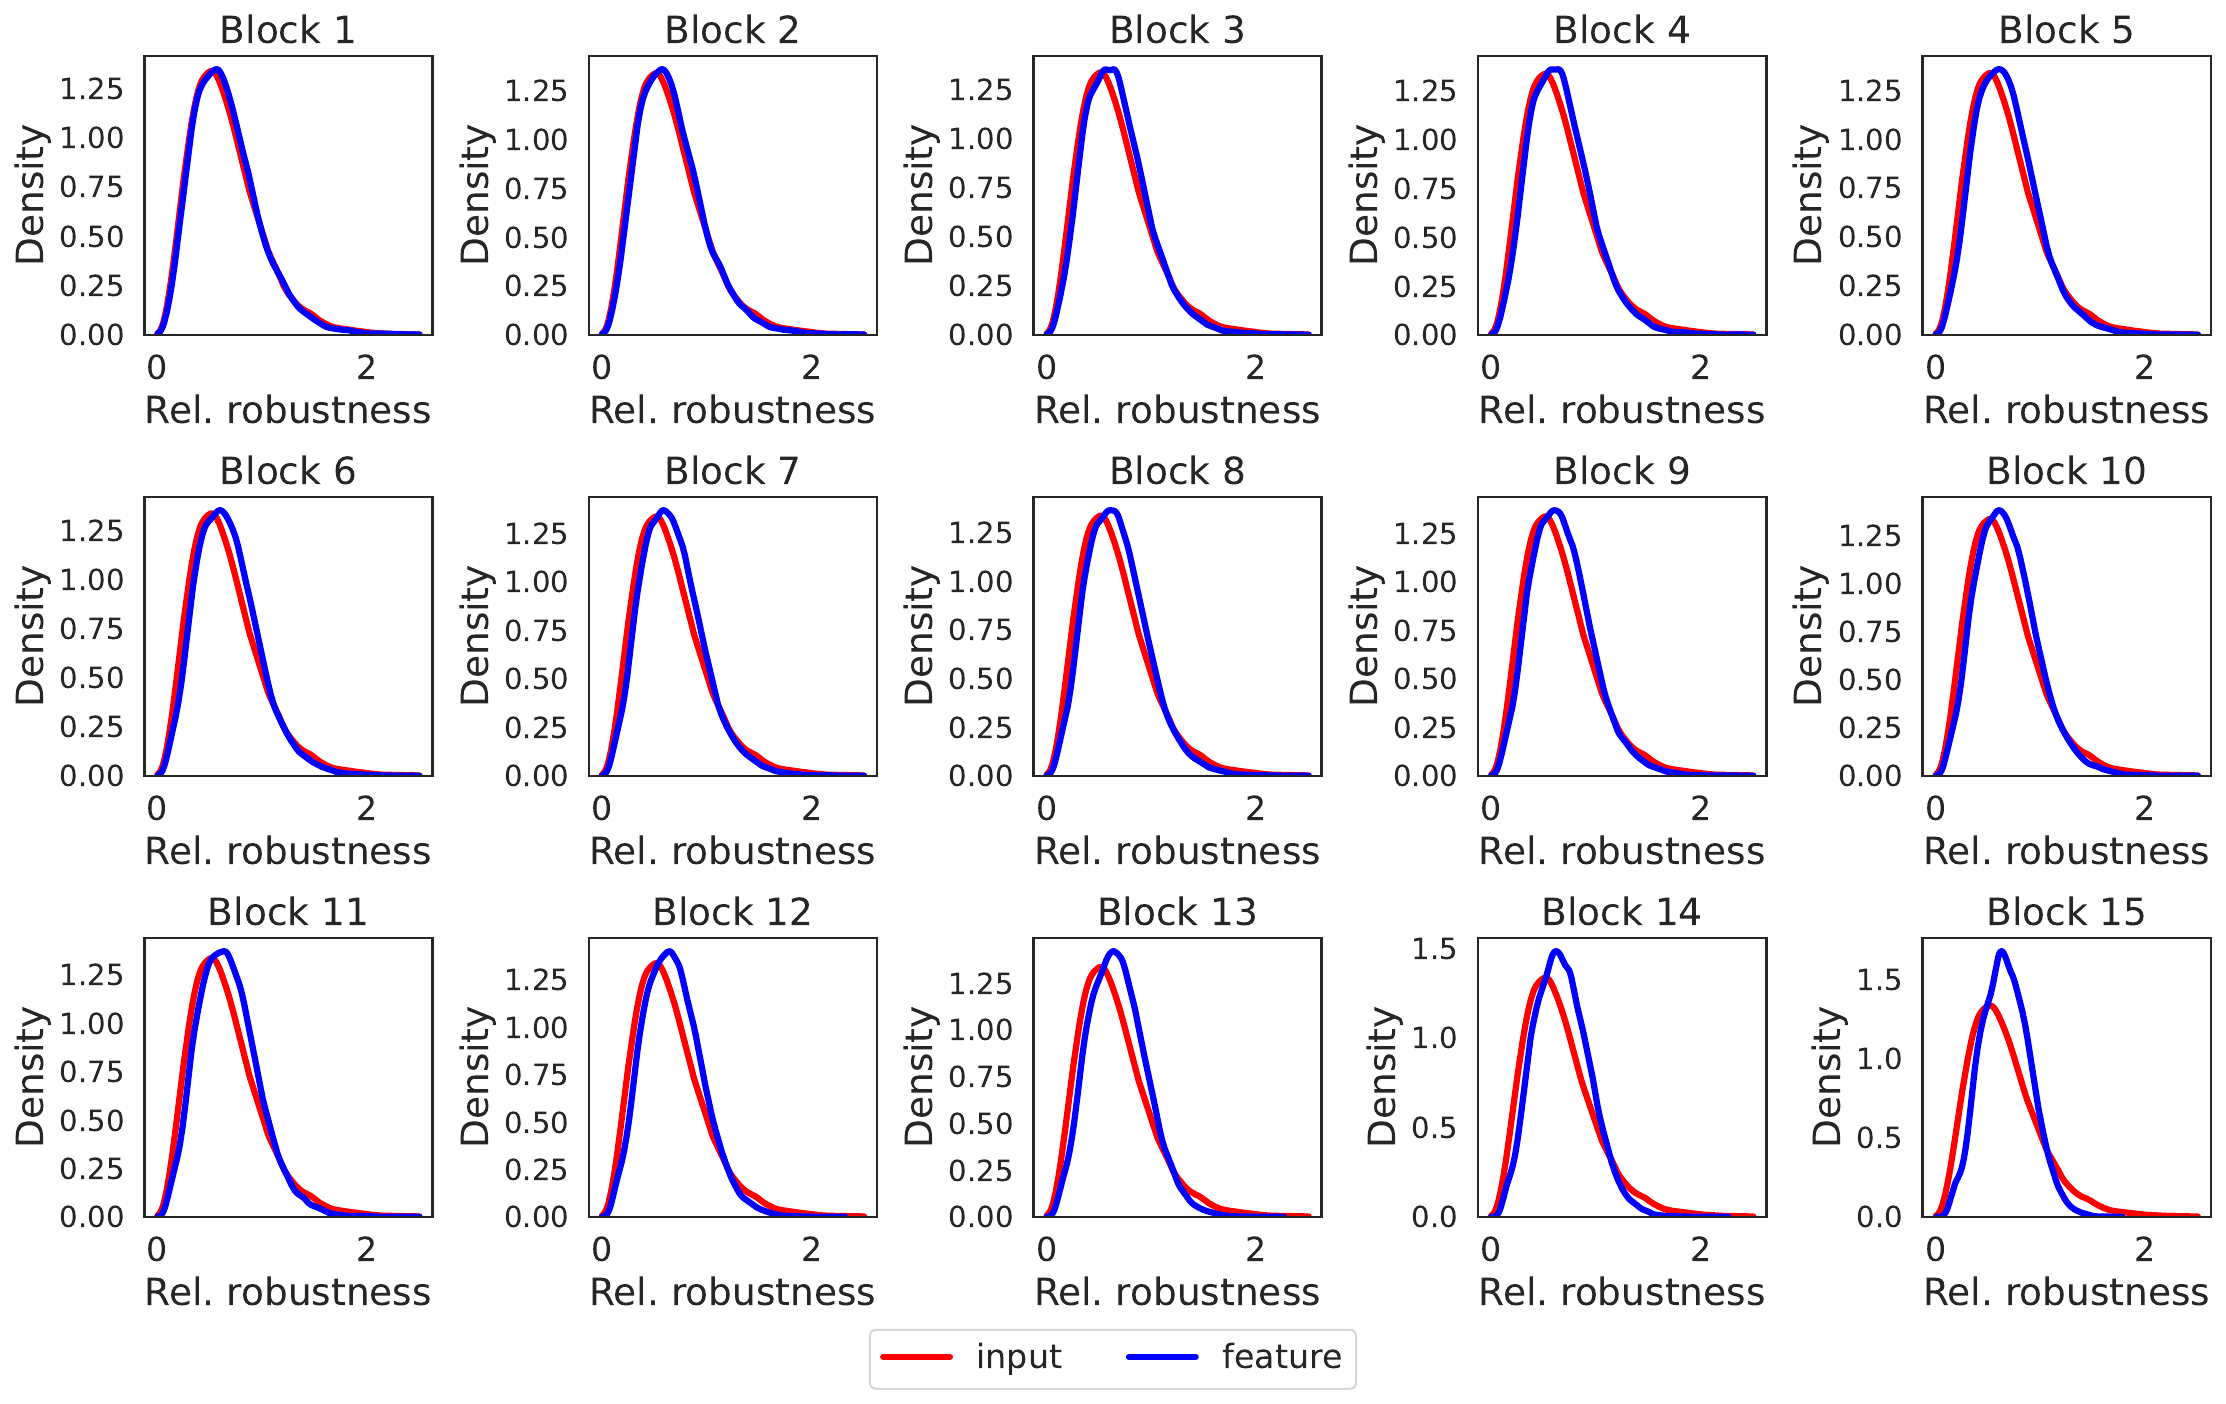}
         \caption{ImageNet}
         \label{fig:vgg_imagenet_acc}
     \end{subfigure}%
     % \vfill
     \begin{subfigure}{0.5\textwidth}
         \centering
         \includegraphics[width=\textwidth]{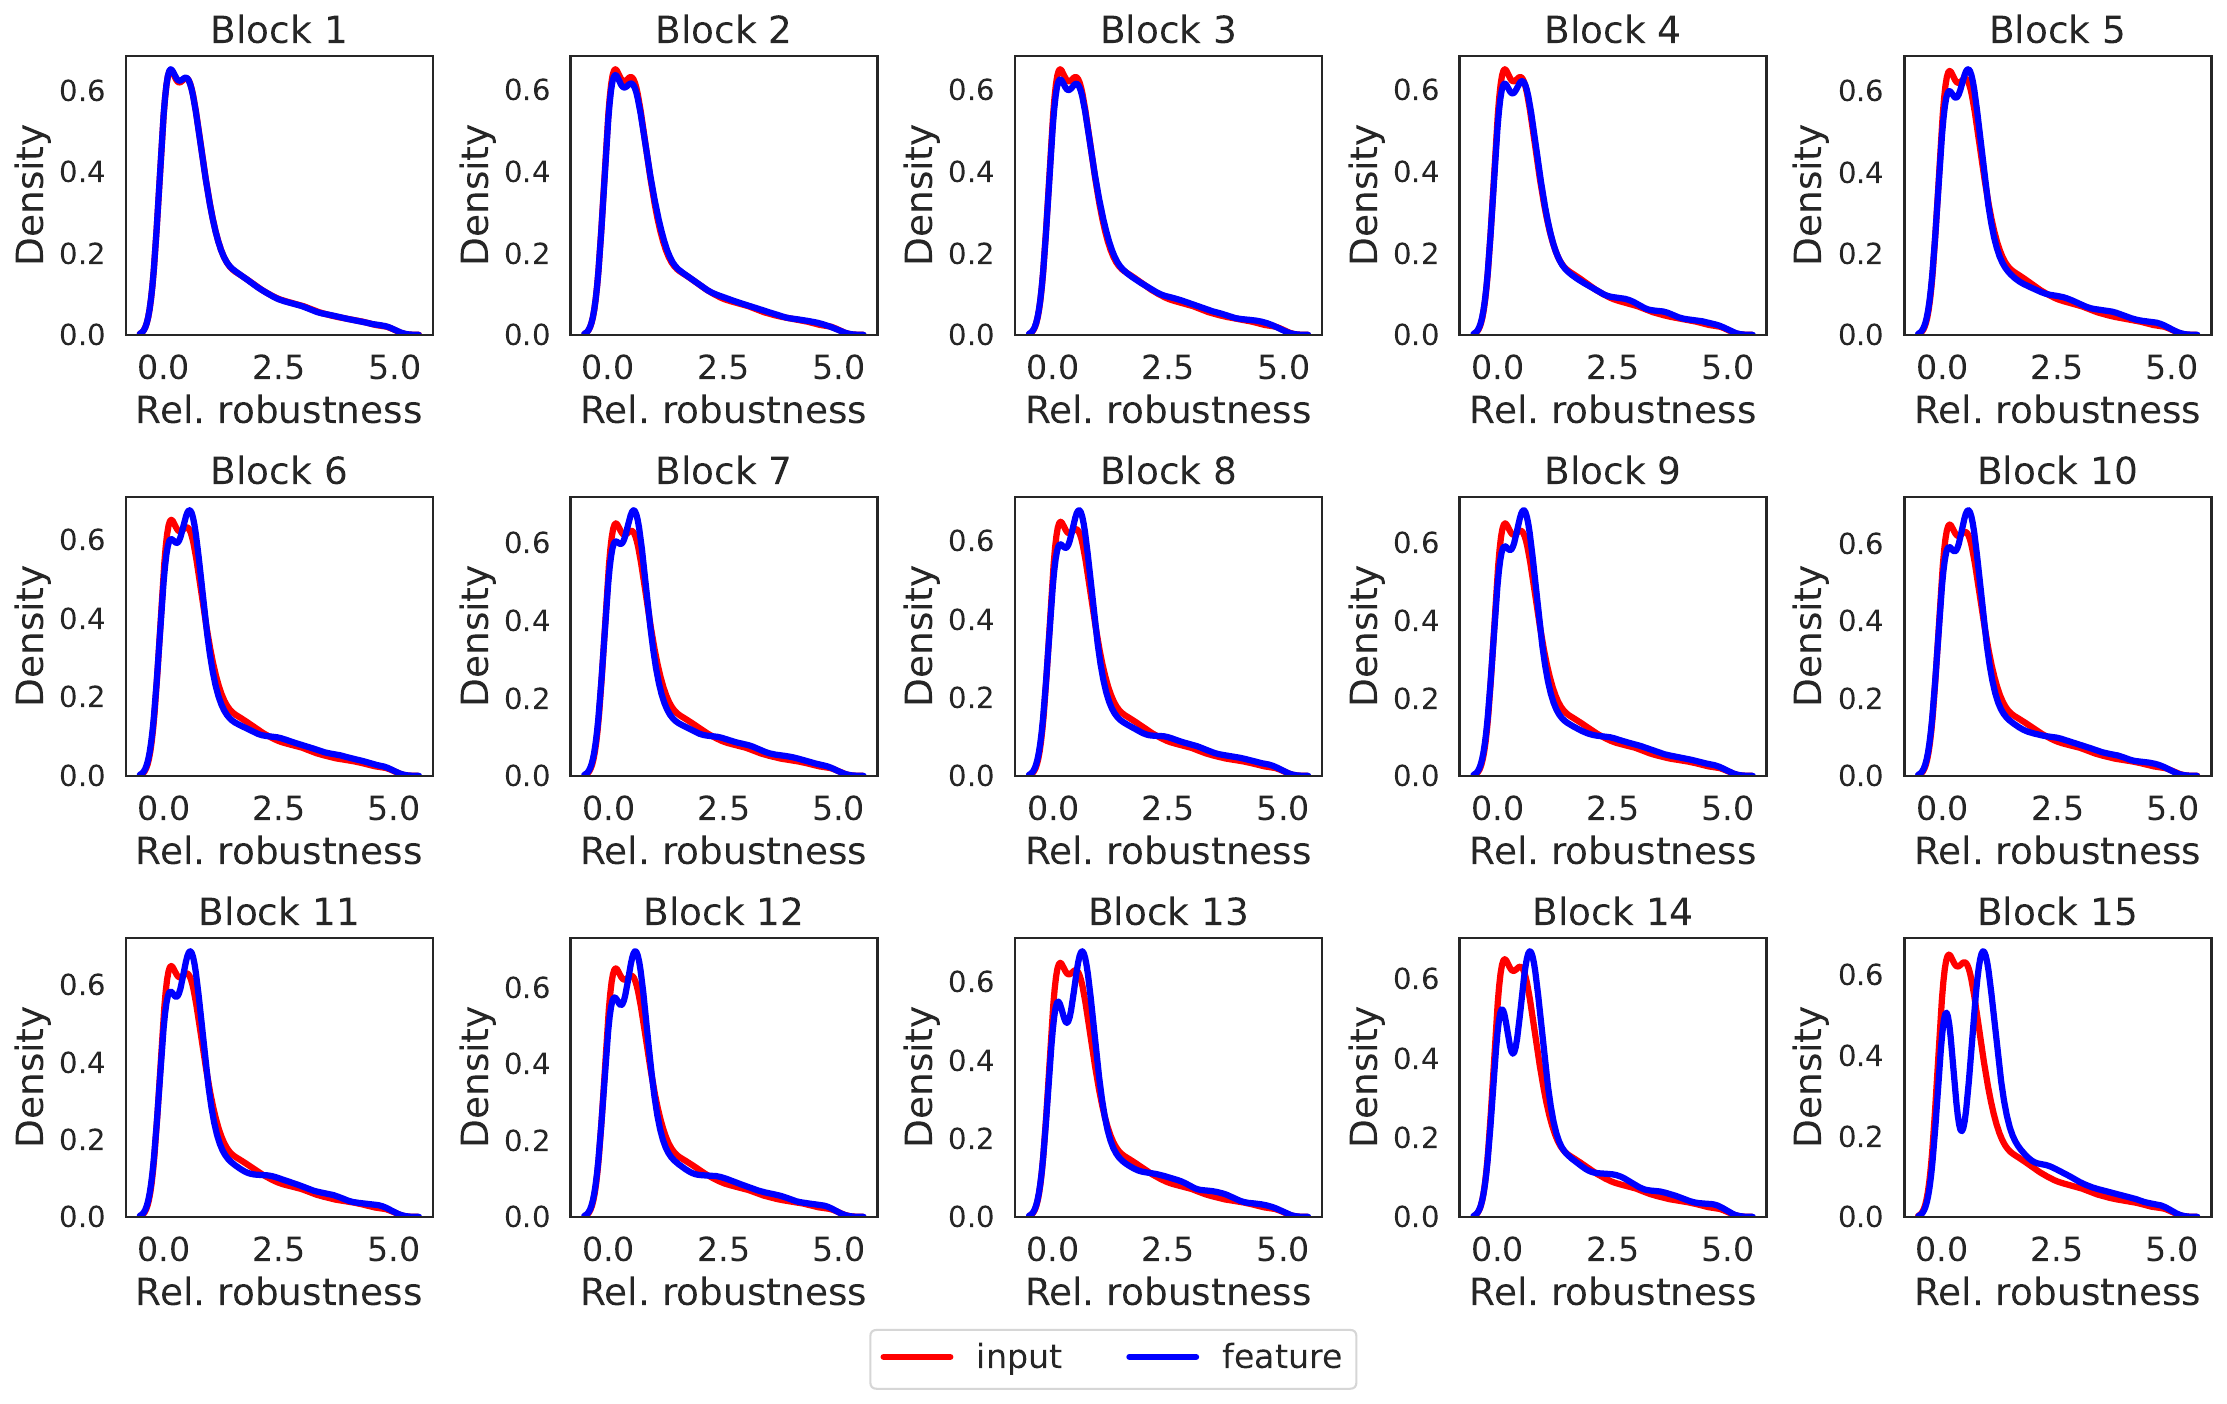}
         \caption{CIFAR10}
         \label{fig:vgg_cifar_acc}
     \end{subfigure}
     \hfill
        \caption{Distributions of the magnitude of the robustness to query-based attacks computed at input and hidden layers of VGG19 on ImageNet/CIFAR10}
        \label{fig:vgg_acc}
\end{figure}
\begin{figure}
     \centering
     \begin{subfigure}{0.5\textwidth}
         \centering
         \includegraphics[width=\textwidth]{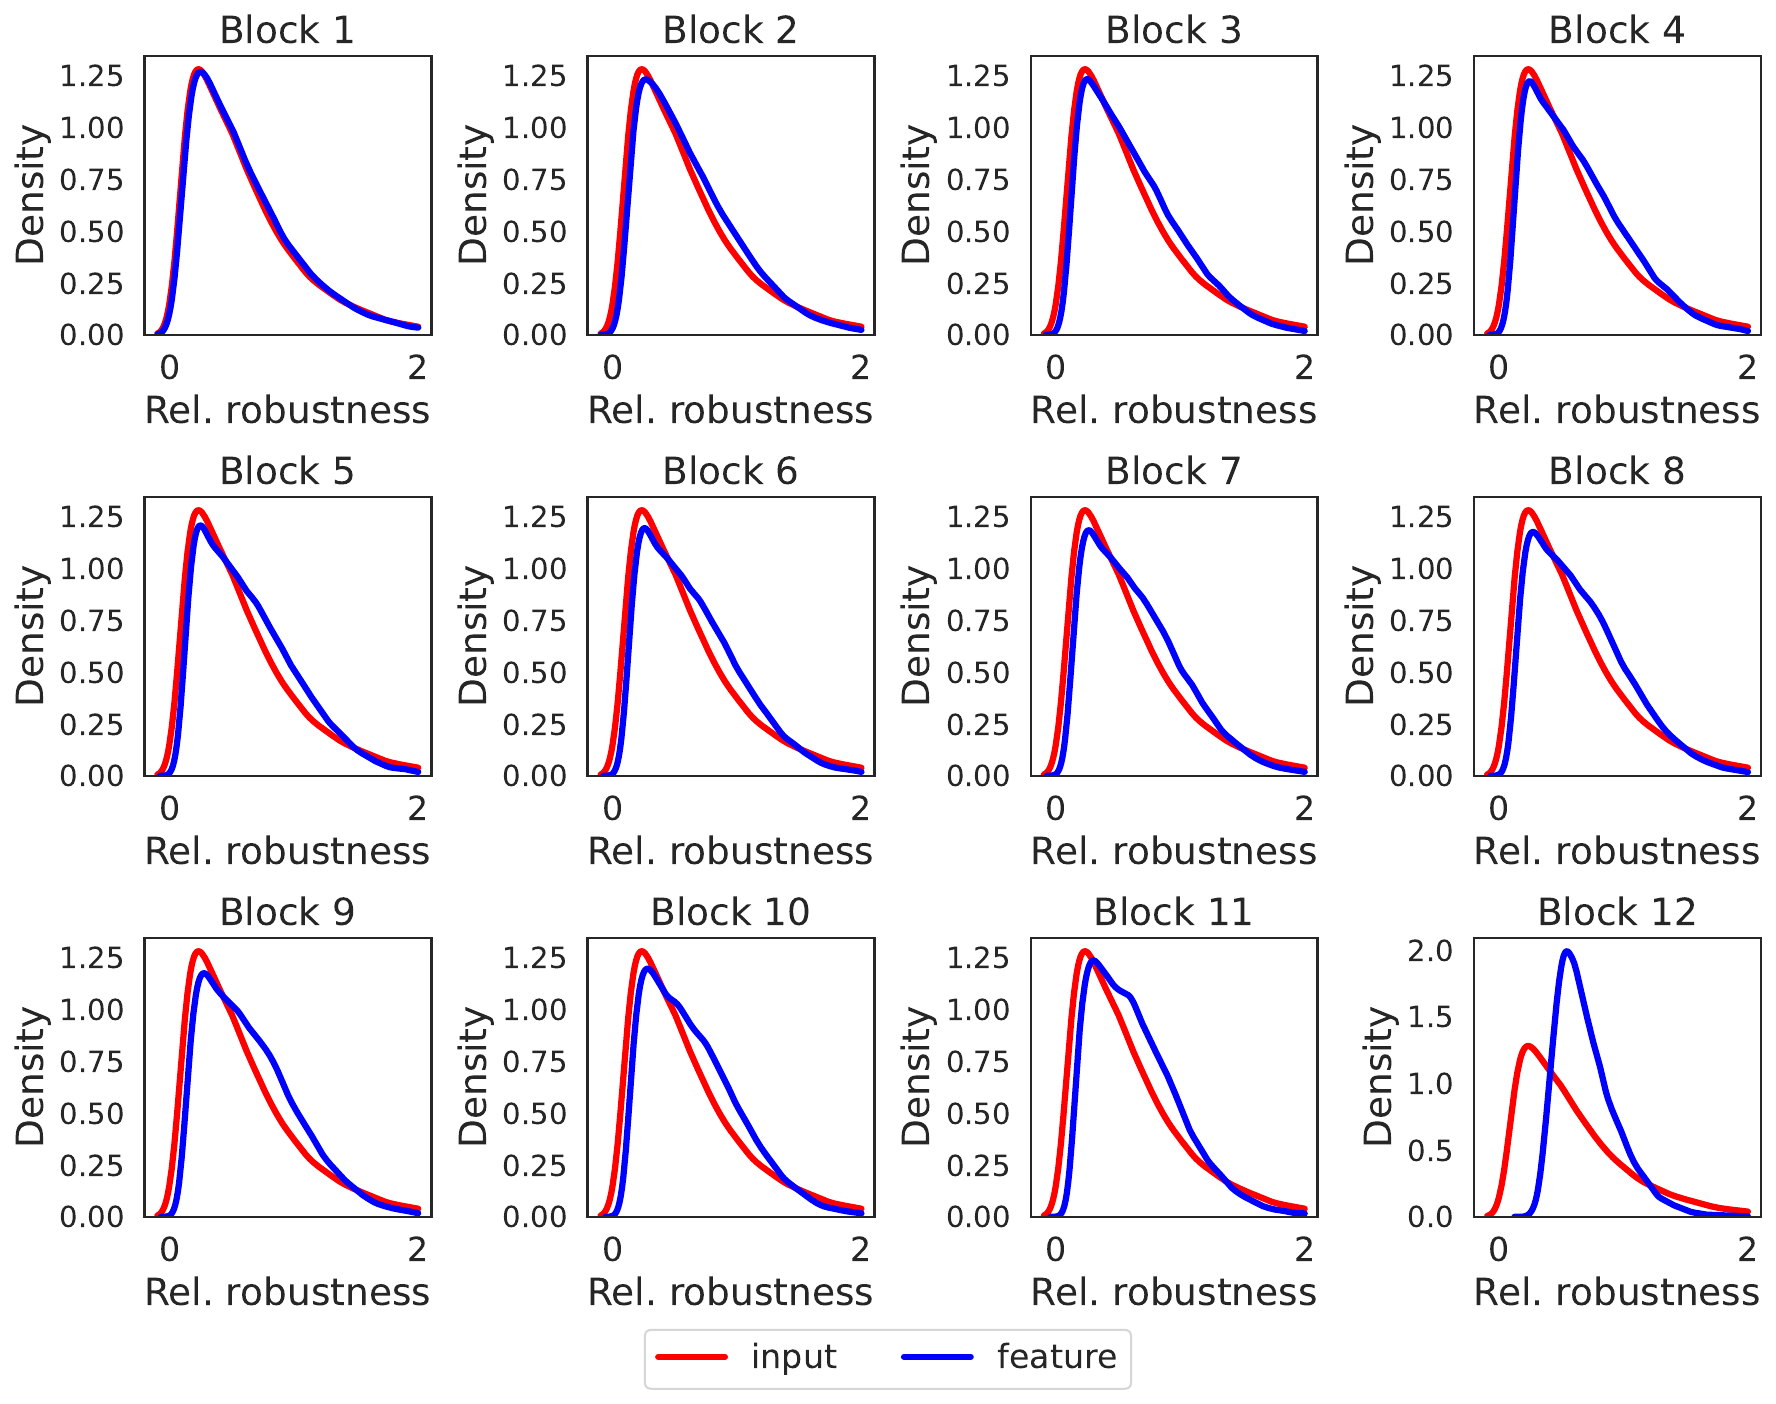}
         \caption{ImageNet}
         \label{fig:vit_imagenet_acc}
     \end{subfigure}%
     % \vfill
     \begin{subfigure}{0.5\textwidth}
         \centering
         \includegraphics[width=\textwidth]{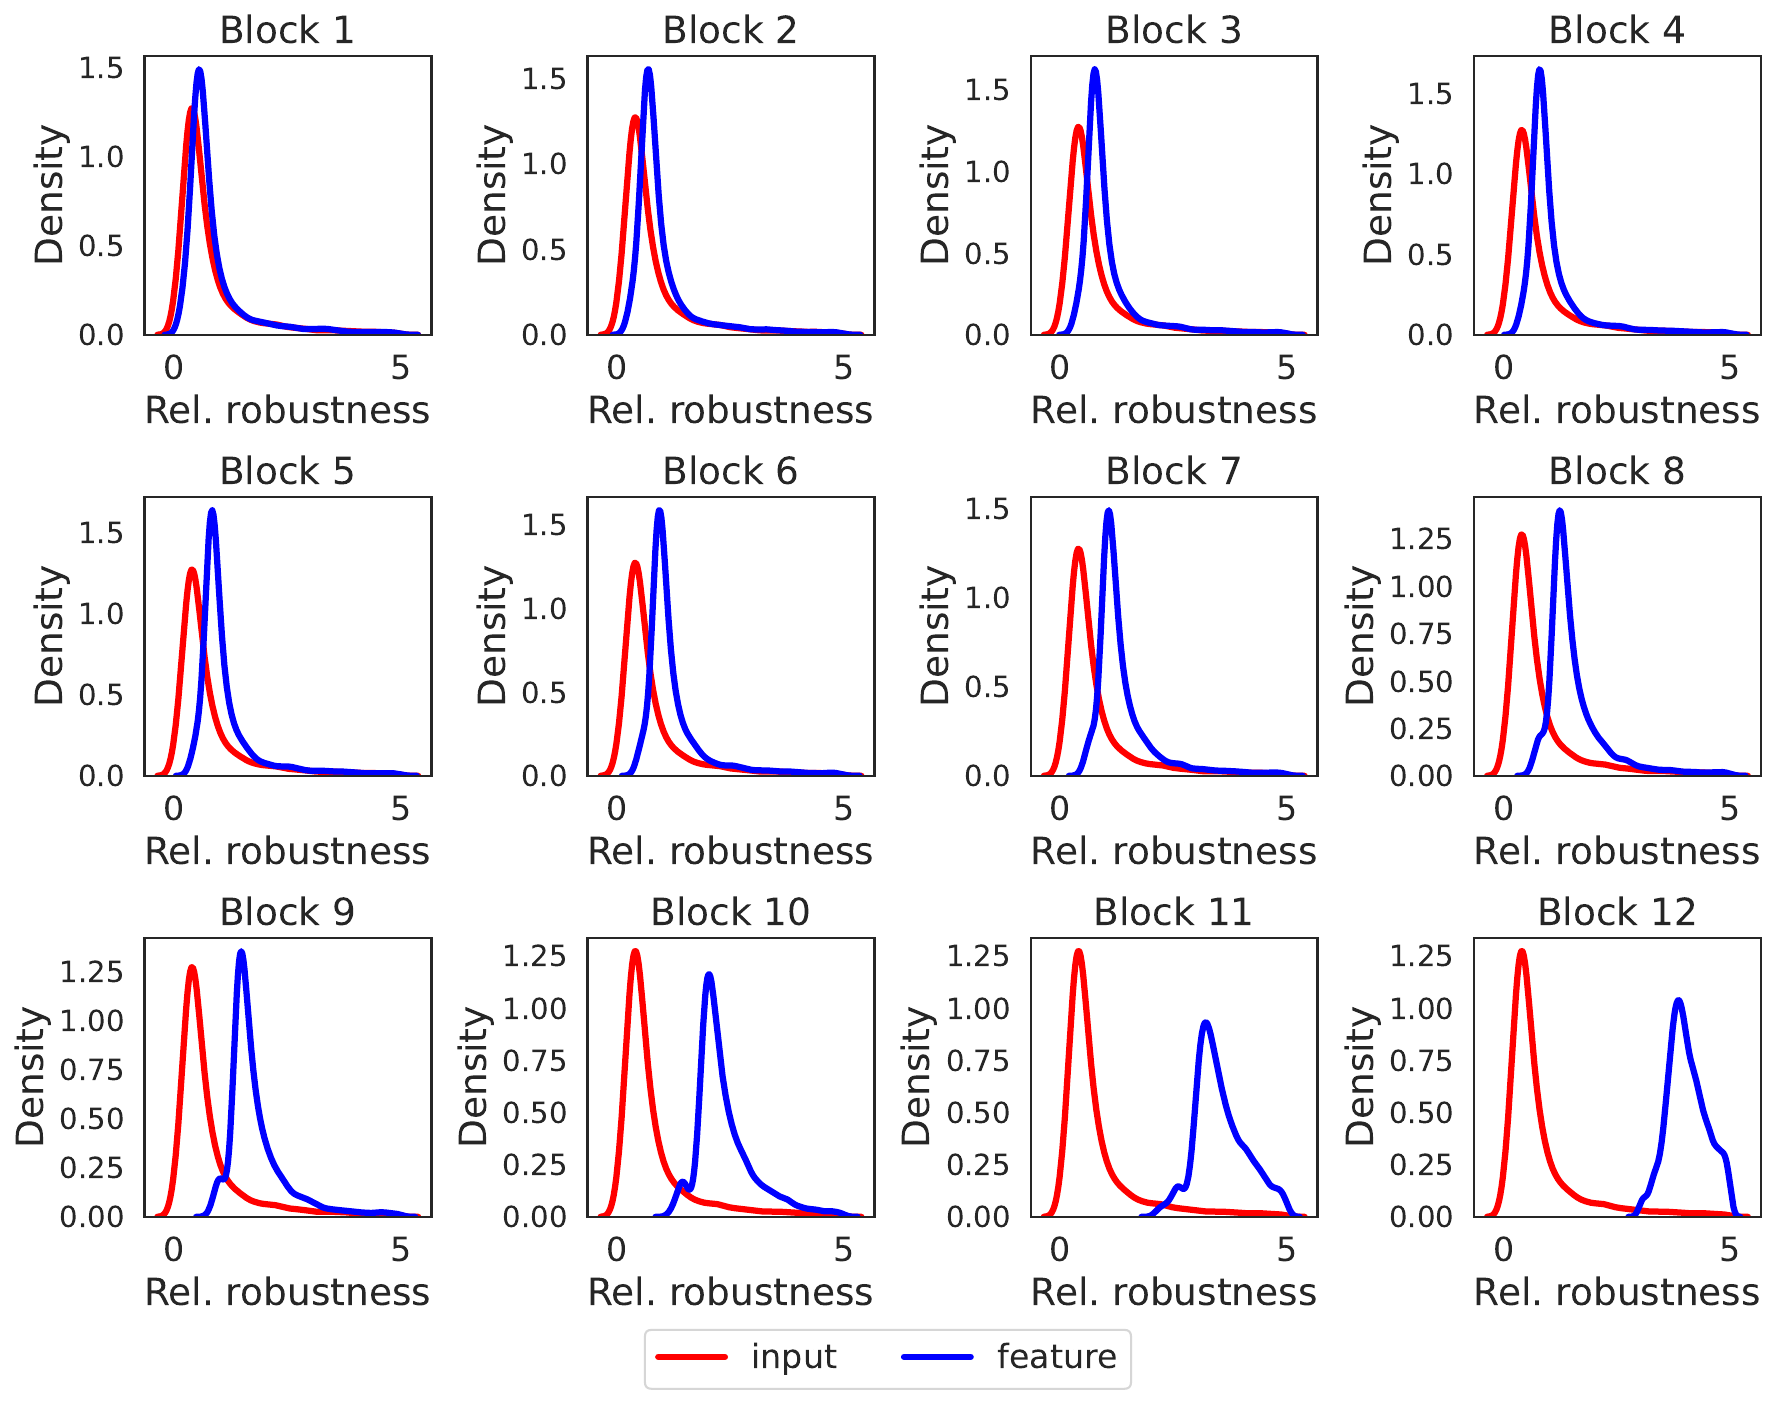}
         \caption{CIFAR10}
         \label{fig:vit_cifar_acc}
     \end{subfigure}
     \hfill
        \caption{Distributions of the magnitude of the robustness to query-based attacks computed at input and selected hidden layers of ViT on ImageNet/CIFAR10}
        \label{fig:vit_acc}
\end{figure}
